# Supplementary material for: Machine learning driven simulated deposition of carbon films: from low-density to diamondlike amorphous carbon
Source: arXiv:2006.09760 ancillary file (2020-11-04)
Supplement: Supplementary file 1 [file supplemental_information.pdf]

# Supplemental Material:

# Machine-learning-driven simulated deposition of carbon films: from low-density to diamond-like amorphous carbon

Miguel A. Caro,[1,2,*] Gábor Csányi,[3] Tomi Laurila,[1] and Volker L. Deringer[4]

[1]*Department of Electrical Engineering and Automation, Aalto University, Espoo, Finland*
[2]*Department of Applied Physics, Aalto University, Espoo, Finland*
[3]*Engineering Laboratory, University of Cambridge, Cambridge CB2 1PZ, United Kingdom*
[4]*Department of Chemistry, University of Oxford, Oxford OX1 3QR, United Kingdom*

(Dated: September 28, 2020)

We attach miscellaneous material supplemental to the main text.

## I. EFFECT OF SUBSTRATE THICKNESS ON GROWTH

GAPs are significantly cheaper than DFT from the point of view of computational cost, but they are still much more expensive than empirical "classical" potentials like Tersoff or EDIP. Hence, while GAPs make these deposition simulations feasible for the first time with the required accuracy, we are still looking at quite expensive simulations. In the interest of saving CPU time, we needed to make a number of compromises. One of them was the choice of a relatively thin initial diamond substrate. Our simulations with this "thin" substrate show partial graphitization of the lower $2 \times 1$ reconstructed diamond surface as the GAP deposition progresses (Fig. 5). To better understand whether the substrate size significantly affects the film growth, we repeated the first stages of the deposition (circa 475 initial impacts) with a thicker substrate. As expected, increasing the number of diamond layers prevents the transfer of kinetic energy from the impact sites required to graphitize the bottom surface of the substrate. However, the characteristics of the grown film at the top surface are virtually the same between "thick" and "thin" substrates, highlighting that the substrate thickness has little or no role on the properties of the grown a-C films once steady-state growth has set in, and only the deposition energy is responsible for the material's characteristics.

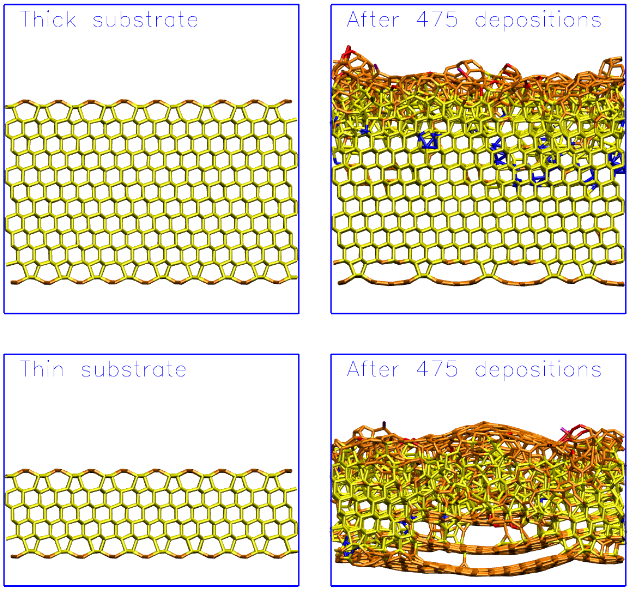


FIG. 1. Initial (111) diamond substrates and state of the substrates after circa 475 depositions (see also Supplementary Material for the initial work).

## II. CHOICE OF TIME STEP

Impacting ions with different energies lead to different maximum velocities in the simulation. Equilibration to the nominal substrate temperature also means that this maximum decreases after impact. To prevent 1) too long atomic displacements between force evaluations and 2) wasting CPU time, we looked at the maximum velocities during and after impact (Fig. 2) and chose the time step accordingly, so that the maximum atomic displacements would stay below 0.1 Å. This means that several time steps were used during different parts of the same deposition event. In addition, more energetic ions implant more kinetic energy into the substrate. Therefore, the equilibration time was also chosen differently for each deposition energy. The different choices are summarized in Table I.

## III. CHARACTERIZATION OF THE THERMAL SPIKE DURING DEPOSITION

In Fig. 3 we show the local and global temperature profiles for a 100 eV deposition event, simulated with and without a thermostat. The incident atom gives rise to a fairly localized thermal spike within the impact region. Since the thermal spike is localized, this justifies using a thermostat applied to all atoms, as opposed to a wall thermostat. The lower panels in the figure depict the global temperature profiles during the 1 ps of MD during which each impact at 100 eV is simulated. We run the same simulation once entirely within a microcanonical (NVE) ensemble and once following our deposition protocol (initial NVE, plus subsequent NVT). It can be seen that most

* mcaroba@gmail.com

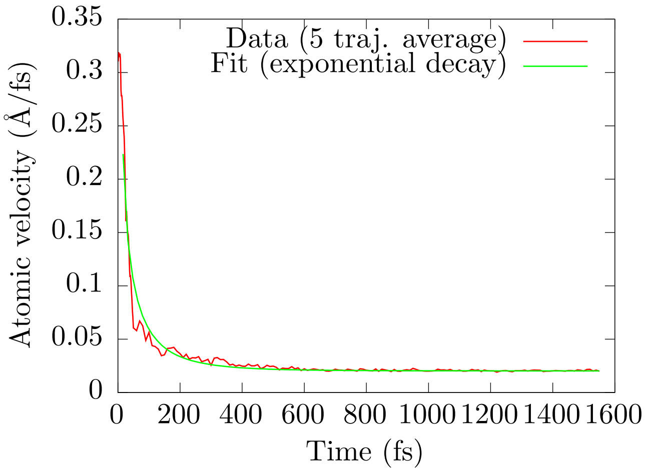


FIG. 2. Maximum velocity registered during atomic deposition (60 eV) with GAP.

of the relaxation takes place during the initial 100 fs. Since the beginning of the NVT dynamics (50 fs at 100 eV) is actually run in the NVE, and the coupling constant of the Nosé-Hoover thermostat (which is switched on after the intial NVE stage) is 100 fs, the thermostat will not introduce significant artifacts into the system dynamics.

## IV. DENSITY PROFILES FOR ALL FILMS

The density profiles for all the films simulated during this study are given in Fig. 4.

## V. DETAILED COHP ANALYSIS FOR 5-C COMPLEXES

COHP and ICOHP (integrated COHP) information for the 5-c complexes characterized in this work (averaged over the 25 studied complexes) is given in Fig. 5.

TABLE I. Variable time steps for the deposition simulations.

| | 1 eV; 300 K | |
|---|---|---|
| Time step | Number of steps | Time |
| 1 fs | 50 | 50 fs |
| 2 fs | 50 | 100 fs |
| | 150 | 0.150 ps |
| | 2 eV; 300 K | |
| Time step | Number of steps | Time |
| 1 fs | 50 | 50 fs |
| 2 fs | 100 | 200 fs |
| | 150 | 0.250 ps |
| | 3 eV – 5 eV; 300 K | |
| Time step | Number of steps | Time |
| 0.5 fs | 100 | 50 fs |
| 1 fs | 20 | 20 fs |
| 2 fs | 100 | 200 fs |
| | 220 | 0.270 ps |
| | 6.5 eV – 10 eV; 300 K | |
| Time step | Number of steps | Time |
| 0.4 fs | 100 | 40 fs |
| 1 fs | 30 | 30 fs |
| 2 fs | 150 | 300 fs |
| | 280 | 0.370 ps |
| | 20 eV; 300 K | |
| Time step | Number of steps | Time |
| 0.15 fs | 200 | 30 fs |
| 0.25 fs | 120 | 30 fs |
| 0.5 fs | 100 | 50 fs |
| 1 fs | 200 | 200 fs |
| 2 fs | 100 | 200 fs |
| | 720 | 0.510 ps |
| | 60 eV; 300 K | |
| Time step | Number of steps | Time |
| 0.1 fs | 200 | 20 fs |
| 0.25 fs | 120 | 30 fs |
| 0.5 fs | 100 | 50 fs |
| 1 fs | 200 | 200 fs |
| 2 fs | 225 | 450 fs |
| | 845 | 0.760 ps |
| | 100 eV; 300 K | |
| Time step | Number of steps | Time |
| 0.1 fs | 200 | 20 fs |
| .25 fs | 120 | 30 fs |
| 0.5 fs | 100 | 50 fs |
| 1 fs | 200 | 200 fs |
| 2 fs | 350 | 700 fs |
| | 970 | 1 ps |

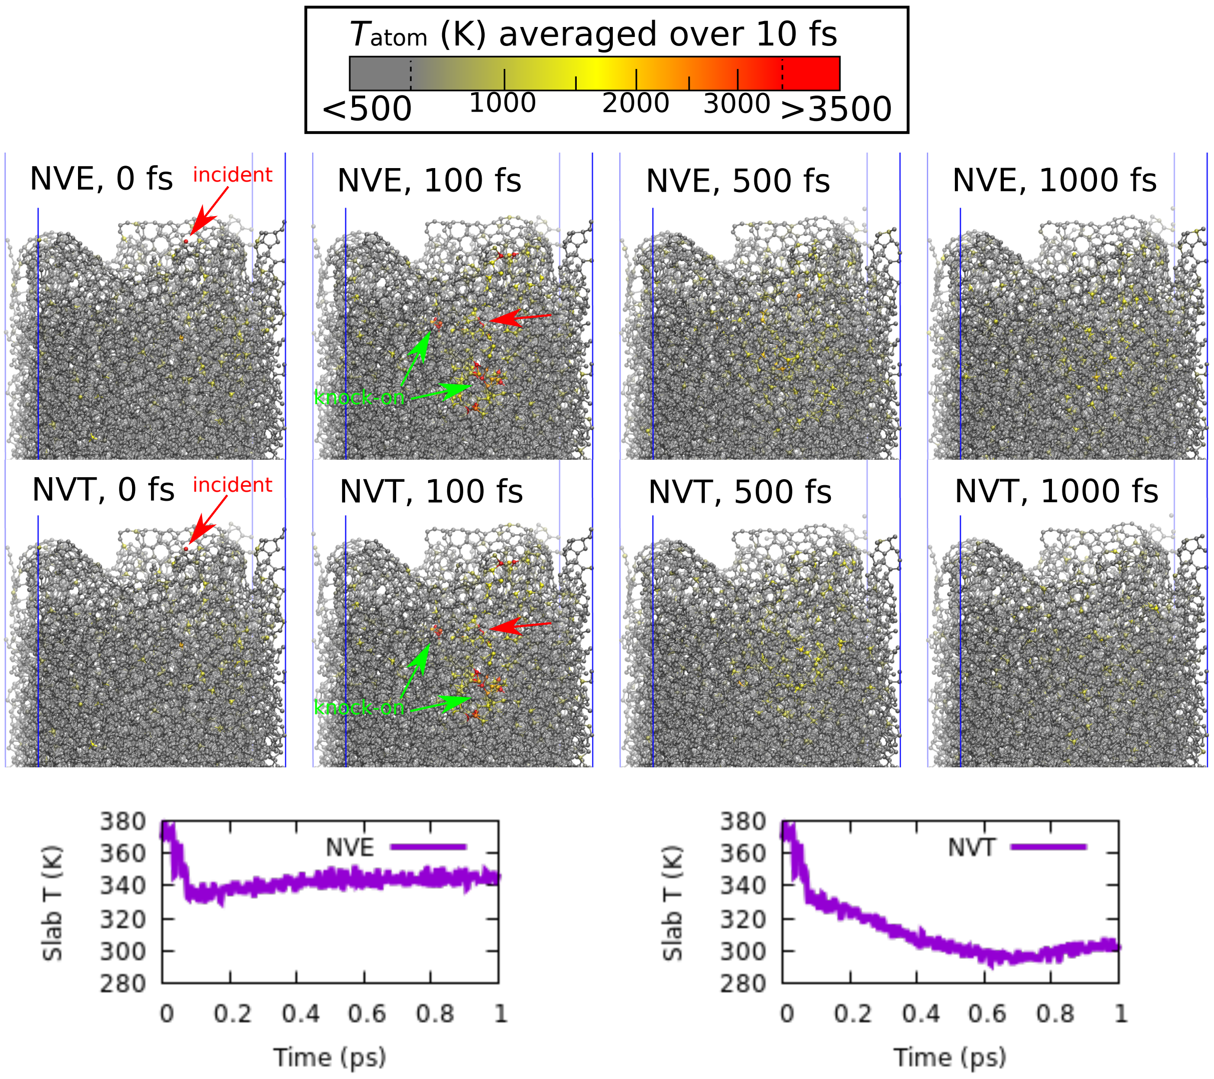


FIG. 3. Thermal spike upon impact and subsequent equilibration for a 100 eV deposition event (the highest energy regime studied in this paper. The local temperatures for the atoms are estimated using a 10 fs averaging window.

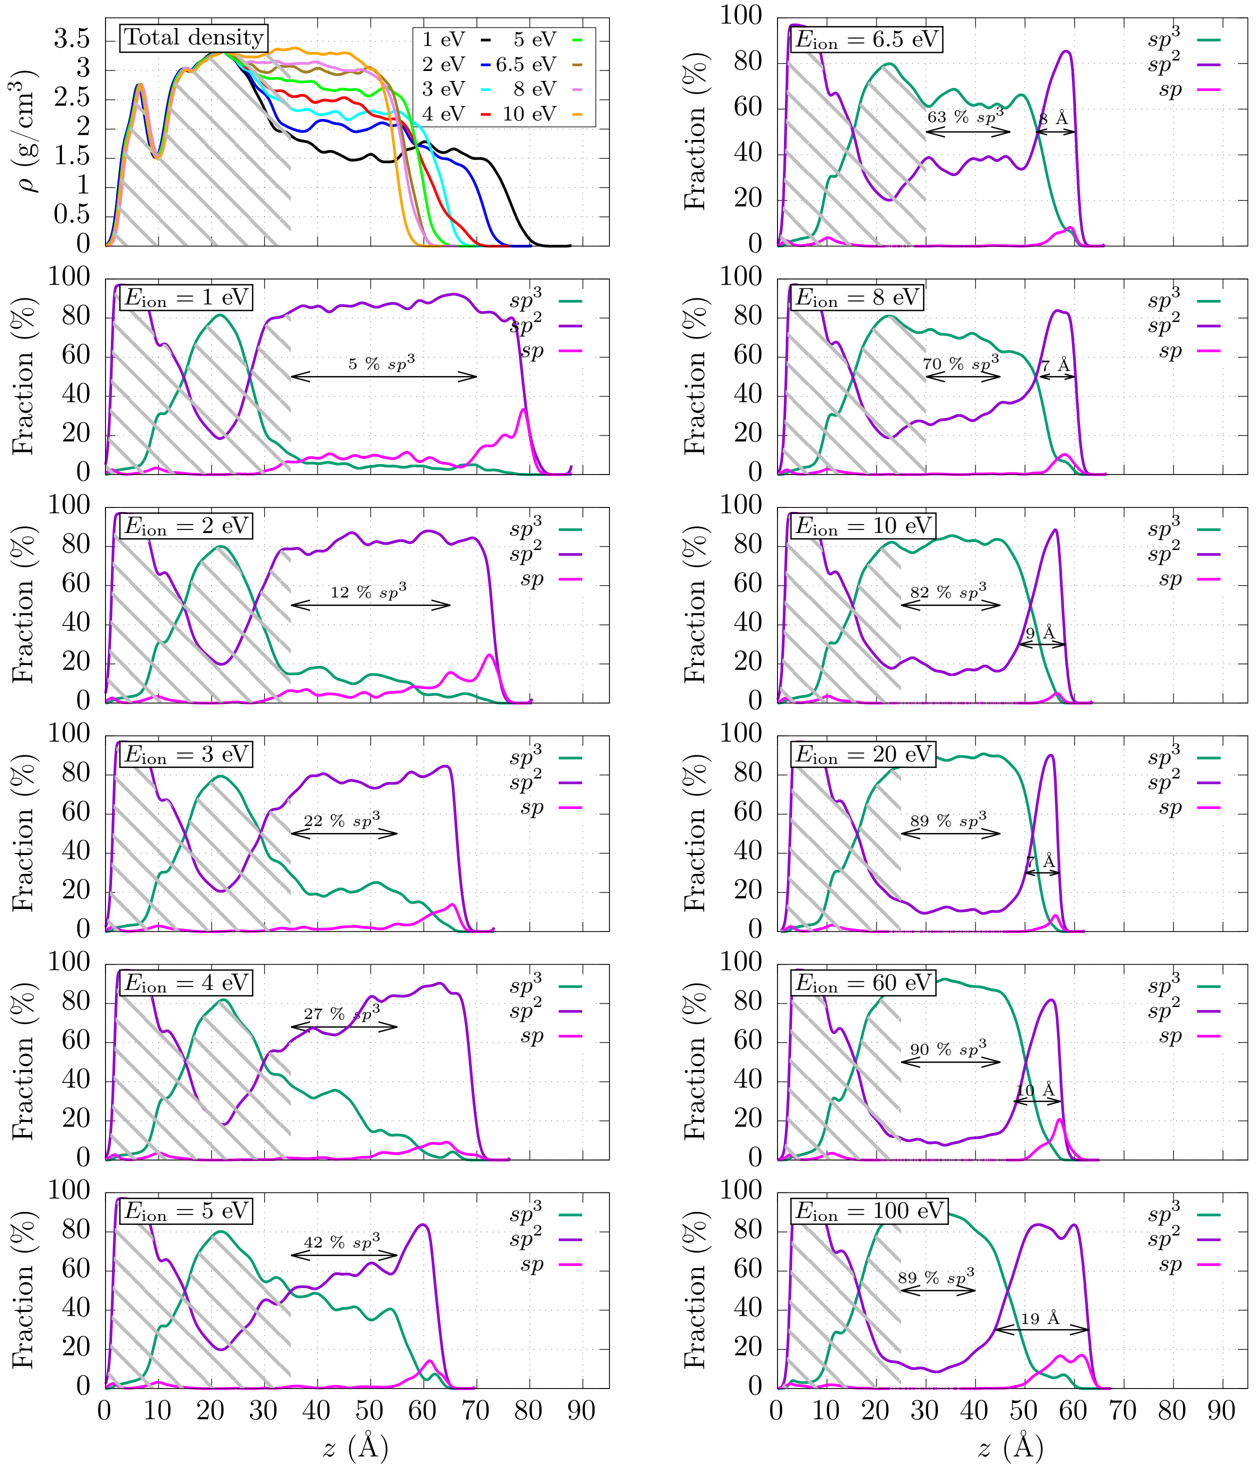


FIG. 4. Mass density profiles and $sp$, $sp^2$ and $sp^3$ fractions for all the films simulated in this work.

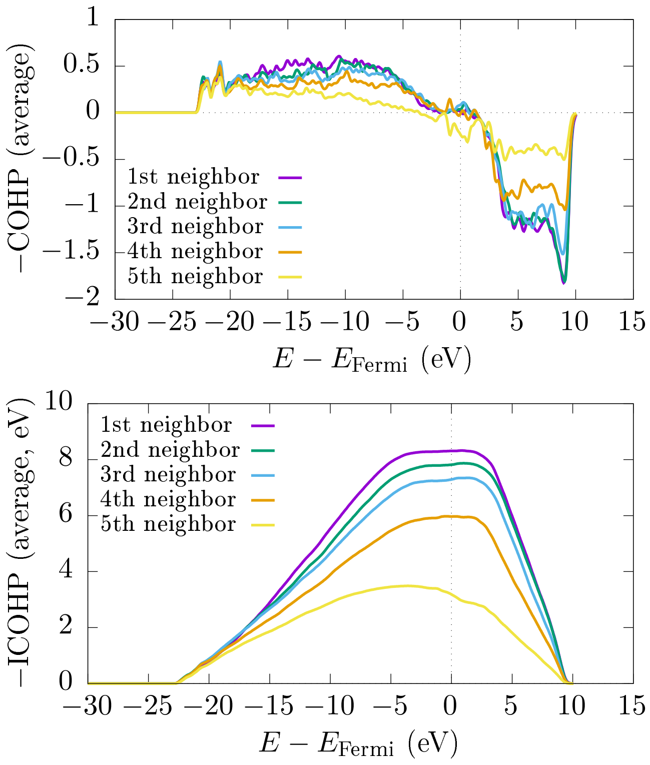


FIG. 5. COHP and ICOHP profiles for 1st to 5th neighbors in the 5-fold coordinated complexes. The curves are averaged over the 25 complexes that we characterized. The upper panel shows the energy-resolved bonding situation: that in the first four neighbor interactions is qualitatively similar to the bonding in diamond but shows a non-bonding, viz. neither stabilizing nor destabilizing interaction (–COHP $\approx 0$) in the region of the Fermi level, which is set as energy zero. In contrast, the 5th neighbor environments entail notable antibonding (–COHP $< 0$) interactions, consistent with a much weaker interaction. The lower panel shows the energy-integrated –COHP curves; the value at the Fermi level is taken to be a measure for the strength of a given bond. Details of the COHP methodology are given in the main text.
